# Supplementary material for: Looped liquid-liquid coexistence in protein crystallization
Source: arXiv:1910.06865 ancillary file (2019-10-15)
Supplement: Supplementary file 1 [file Supplemental_Material.pdf]

# Supplemental Material for “Looped liquid-liquid coexistence in protein crystallization”

(Dated: October 4, 2019)

## CONTENTS

|                                                                                      |    |
|--------------------------------------------------------------------------------------|----|
| I. Description of supplementary movies                                               | 1  |
| II. Materials and Methods                                                            | 1  |
| A. Patchy shape simulation model                                                     | 1  |
| B. Crystalline order parameter                                                       | 2  |
| C. Liquid-liquid phase coexistence                                                   | 2  |
| D. Estimation of entropy contributions                                               | 2  |
| E. Determination of the liquid-solid surface tension                                 | 2  |
| F. Simulation code                                                                   | 3  |
| G. Compute resources and data management                                             | 3  |
| III. Phase behavior of the patchy shape model                                        | 3  |
| A. Gibbs free energy surface (GFES) from well-tempered Metadynamics (WTMetaD)        | 3  |
| 1. Extrapolation of the GFES to nearby state points                                  | 3  |
| 2. Location of minima and reweighting of the GFES                                    | 5  |
| B. Thermodynamic integration of the Helmholtz free energy                            | 5  |
| 1. Liquid-liquid coexistence from thermodynamic integration of the equation of state | 5  |
| C. Critical points                                                                   | 8  |
| D. Fluid-solid coexistence                                                           | 8  |
| 1. Solid free energy using the Frenkel-Ladd method                                   | 9  |
| 2. Equation of state from isothermal-isobaric (NPT) simulations                      | 9  |
| 3. Fluid-solid equilibrium from Gibbs-Duhem integration                              | 9  |
| IV. Prenucleation motifs in the high-density liquid phase                            | 10 |
| V. Characterization of the surface tension                                           | 11 |
| References                                                                           | 11 |

## I. DESCRIPTION OF SUPPLEMENTARY MOVIES

**Movie 1** shows a simulation trajectory of crystallization of  $N = 8192$  particles at  $\varepsilon_c = 0.31$ ,  $\varepsilon_l/\varepsilon_c = 0.6$ ,  $\phi = 0.2$ , where we only show particles with crystalline order parameter  $\theta_c \geq 60$ , and color by the value of  $\theta_c$ .

**Movie 2** shows a single nucleation event at the same parameters as Movie 1. Here, particles are shown as spheres only if they are part of the five-fold ring motifs and are colored according to the age of the cluster they participate in (from bright to dark). Particles on the surface of the nucleus appear bright, indicating that they integrate into existing ring clusters through monomeric attachment rather than attachment of clusters, *i.e.*, according to classical nucleation and growth.

## II. MATERIALS AND METHODS

### A. Patchy shape simulation model

We parameterize the model using the crystallographic unit cell of wild-type rubredoxin (PDB 1BRF<sup>1</sup>), which includes four particles in orthorhombic,  $P2_12_12_1$  symmetry (Fig. 1, main text), the most common of protein space groups. By placing a cut-off of 0.55 nm on the distance between atom-atom contacts in the unit cell, we identify the

three protein-protein interfaces with the largest surface area.<sup>2</sup> We use a program based on BioJava's **CrystalBuilder**<sup>3</sup> to identify the three largest unique interfaces of the rubredoxin crystal structure (1BRF) within a cut-off of 0.55 nm. On a molecular level, the first two interfaces correlate with hydrophobic patches on the protein surface, while the third interface involves an electrostatic contact mediated by a conformation change.<sup>4</sup> We model the shape of rubredoxin as a rigid body of 414 spheres defined by the positions and van-der-Waals diameters  $\sigma_i$  of the constituent atoms with bound hydrogens.<sup>5</sup> The spheres interact with a shifted Weeks-Chandler-Anderson (WCA) interaction of unit strength,  $U_{SWCA}(r) \equiv U_{SLJ} + k_B T$  with  $U_{SLJ}(r) = 4k_B T \left\{ [\sigma/(r - \Delta)]^{12} + [\sigma/(r - \Delta)]^6 \right\}$ ,  $\Delta = (1/2)(\sigma_i + \sigma_j) - \sigma$ , cut off at  $2^{1/6}\sigma + \Delta$ .<sup>6</sup> We choose  $\sigma = 0.25$  nm for the range of the interaction, and set  $k_B T = 1$ . We term interactions between interfaces occurring in the crystallographic structure as *native*, and interactions between interfaces that do not occur in the crystal as *non-native* (Fig. 1b). The non-native interactions mediate isotropic or liquid-like interactions, whereas the native interactions provide the directionality needed to stabilize the crystal structure. The two types of attractive interactions are characterized by interaction strengths  $\varepsilon_l$  and  $\varepsilon_c$ , respectively. The native interaction strength can be interpreted as an inverse reduced temperature  $T^* \equiv T/\varepsilon_c$ . For simplicity, we assume that the strength of native and non-native interactions is independent of the type of interface. We chose the shifted Lennard-Jones potential  $U_{SLJ}(r)$  to represent all attractive interactions. We choose the range of interaction  $\sigma = 0.25$  nm of the shifted Lennard-Jones interaction as a value comparable to the size of a solvent molecule ( $d_{H_2O} \approx 0.28$  nm) and commensurate with the width of the attractive well in atomistic molecular dynamics simulations of the crystal contacts.<sup>4</sup> We assign unit mass to the constituent spheres of the rigid bodies and choose a Molecular Dynamics time step of  $\Delta t = 0.005$ .

### B. Crystalline order parameter

To characterize the average amount of crystalline order, we introduce the quantity  $\theta_c \equiv -\langle U_c \rangle / \varepsilon_c N k_B T$ , which is proportional to the number of contacts per particle that are compatible with the target structure.

### C. Liquid-liquid phase coexistence

We ran well-tempered metadynamics simulations at select  $(P^*, \varepsilon_c)$  points on the liquid-liquid coexistence curve to determine the location of the minima on the Gibbs free energy surface, using three collective variables  $\theta_c$ ,  $\theta_n$  and  $\phi$ . For examples of the free energy surface and details on the analysis method, see III A. We validated the location of the metastable liquid-liquid coexistence using thermodynamic integration of the Helmholtz free energy, see Sec. III B 1. We describe the estimation of the critical points in Sec. III C.

We calculated the Gibbs free energy to infer the fluid-solid coexistence curve. To obtain an initial point on the fluid-solid coexistence curve, we integrated the solid free energy using the Frenkel-Ladd method,<sup>7,8</sup> and obtained smooth boundaries by integrating the generalized Clausius-Clapeyron equation using Hamiltonian Gibbs-Duhem integration,<sup>9,10</sup> see Sec. III D 3.

### D. Estimation of entropy contributions

To estimate the entropy contributions in Fig. 2d, we computed the pairwise excess translational entropy,<sup>11</sup>

$$S_2 = -2k_B T \rho \int_0^\infty dr r^2 [g(r) \ln g(r) - g(r) + 1], \quad (1)$$

from the radial distribution function  $g(r)$ , and the potential energy  $U$  for all frames of the biased (well-tempered metadynamics) simulations with  $N = 256$  walkers. We then binned and averaged these quantities according to the values of the collective variables  $\phi$ ,  $\varepsilon_c$  and  $\varepsilon_l$  and used interpolation to extract  $S_2$  and  $U$  in the LDL and HDL basins of the Gibbs free energy surface. The rotational contribution to the entropy difference  $\Delta S$  between two states is  $\Delta S_{\text{rot}} \equiv \Delta S - \Delta S_2 - \Delta S_{\text{ideal}}$ , where  $\Delta S_{\text{ideal}} = k_B \ln(V_2/V_1)$ .

### E. Determination of the liquid-solid surface tension

To measure the liquid-solid surface tension  $\gamma$  in simulation, we refined Gasser et al.'s method, which they used to analyze colloidal suspensions.<sup>12</sup> We assume that for small areas, the distribution  $P(A) \propto \exp[-\beta\gamma A + \mathcal{O}(V)]$  of

nuclei area  $A$  follows an exponential distribution. The method assumes a generalization of the free energy of classical nucleation theory to ellipsoidal nucleus shapes. For every nucleus, we calculated the area from the half-axes  $a_i \equiv \sqrt{w_i}$  of the inertia ellipsoids, where  $w_i$  are the eigenvalues of the gyration tensor. We identified nuclei by their matching nearest-neighbor bond vectors,<sup>13,14</sup> with a maximum difference of  $\Delta r = 0.6$  nm between the metrics of two similar environments. Fig. 9 shows a typical distribution of nuclei area together with a fit to an exponential distribution.

## F. Simulation code

We perform GPU-accelerated simulations in the isothermal constant volume (NVT) and constant pressure (NPT) ensembles using HOOMD-blue.<sup>15–17</sup> We use `md.integrate.nvt()` and `md.integrate.npt()`,<sup>18</sup> which implement symplectic and explicitly time-reversible integration methods<sup>19,20</sup> for these ensembles. We support rigid bodies through the symplectic quaternion scheme of Miller *et al.*<sup>21,22</sup>

## G. Compute resources and data management

We performed production runs on the Summit supercomputer at the Oak Ridge National Laboratory, using up to 1500 nodes (9000 GPUs) at a time, to simulate the model over  $4.5 \times 10^7$  molecular dynamics time steps. We take advantage of unified memory support in HOOMD-blue to enable multi-GPU execution on three GPUs of the same compute node for every state point.<sup>23</sup> We ran NPT phase diagram screens and exploratory simulations on the Titan supercomputer at Oak Ridge National Laboratory. Early exploratory simulations used the xStream GPU cluster at Stanford University and the Bridges GPU cluster at Pittsburgh Supercomputing Center.

We organize our data in a `signac` workspace.<sup>24,25</sup> All simulation data and scripts are available at (see **Data availability**). For the well-tempered metadynamics simulations (Sec. III A), we manage job submissions on Summit using the `signac-flow` tool.

# III. PHASE BEHAVIOR OF THE PATCHY SHAPE MODEL

## A. Gibbs free energy surface (GFES) from well-tempered Metadynamics (WTMetaD)

We carry out WTMetaD simulations<sup>26,27</sup> using the `metadynamics-plugin`<sup>28,29</sup> for HOOMD-blue. We sample in the NPT ensemble, and calculate the GFES as a function of three collective variables: the number density of proteins  $\rho$ , the crystal order parameter  $\theta_c \equiv -U_c/N\varepsilon_c$ , and the liquid order parameter  $\theta_l \equiv -U_l/N\varepsilon_l$ . In sampling 1024 proteins, we use a WTMetaD temperature  $\Delta T = 500 T$ , characteristic of the observed height of free energy barriers between the liquid phases, or  $\Delta T/N = 2.048 T$ . We deposit multivariate Gaussians of standard deviation  $\sigma_\rho = 0.01$ ,  $\sigma_c = \sigma_l = 2.5$  and height  $W = k_B T$  every 10 000 MD time steps ( $\delta t = 5 \times 10^{-3}$ ). We sample using  $M = 256$  walkers, with each walker using 3 GPUs, *i.e.* using a total of 768 GPUs simultaneously per state point on the coexistence curve.

We start from disordered, dilute initial conditions. To initially randomize the positions of the walkers in collective variable space, we equilibrate the system for  $5 \times 10^5$  MD steps without bias, and then for another  $5 \times 10^5$  steps with bias accumulation. Subsequently, we reset the bias potential to zero and then sample for  $4.5 \times 10^7$  MD time steps. Most walkers sample the liquid–liquid coexistence, performing several round-trips between the low density and high density basins (Fig. 1). Depending on the state point, some walkers also sample the crystalline phase. However, escapes from the crystal minimum are rarely observed for the chosen sampling time and value of  $\Delta T$ .

### 1. Extrapolation of the GFES to nearby state points

The bias potential  $V \equiv V(\theta_c, \theta_l, \rho)$  thus obtained defines the GFES through the following relationship,<sup>27</sup>

$$G = -\frac{\Delta T + T}{T} V. \quad (2)$$

Fig. 2 shows a volume rendering (using `ipyvolume`)<sup>30</sup> of the three-dimensional GFES, which indicates at least two minima. Our goal is to identify the metastable liquid minima using the condition of equal Gibbs free energy, by extrapolating the GFES from a statepoint  $(\varepsilon_{s,0}, \varepsilon_{n,0}, P_0^*)$  to a nearby statepoint  $(\varepsilon_c, \varepsilon_l, P^*)$  at coexistence. We

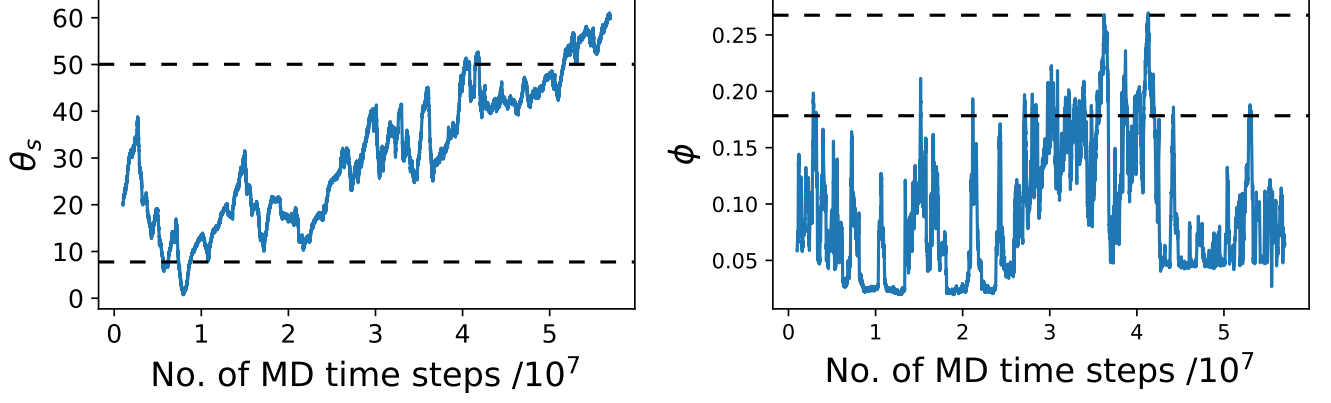

FIG. 1. Trajectory of a single walker in a simulation of  $M = 256$  WTMetaD walkers with  $N = 1024$  proteins at  $\varepsilon_c = 0.37$ ,  $\varepsilon_l/\varepsilon_c = 0.5$  and  $P^* = 0.039776$ , showing sampling of the low-density fluid and the metastable liquid states in the collective variables  $\theta_c$  (crystalline order parameter) and  $\phi$  (density). The values of  $\theta_c$  and  $\phi$  for the low- and high-density liquids are indicated by dashed horizontal lines.

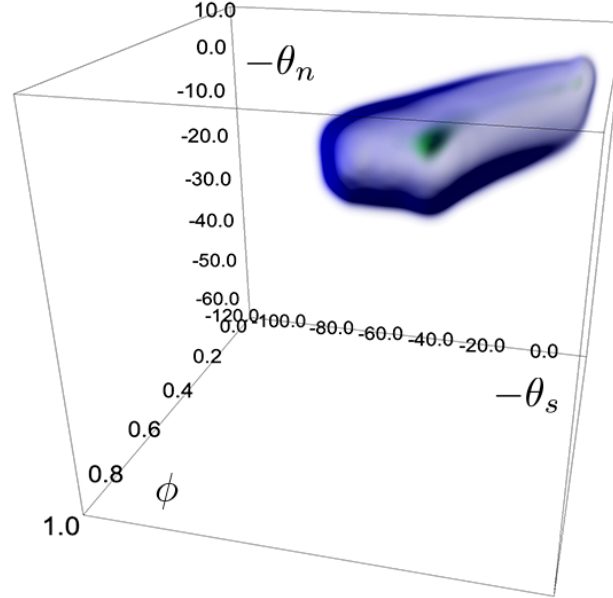

FIG. 2. Volume rendering of the GFES obtained with WTMetaD at  $\varepsilon_c = 0.325$  and  $P^* = 0.5$ , as a function of the collective variables  $\theta_c$ ,  $\theta_l$  and  $\phi$ . Local minima are highlighted in green. The analysis of Sec. III A 2 reveals the metastable liquid minima.

expand  $G$  to first order in these parameters, and exploit the fact that the collective variables  $\theta_c$ ,  $\theta_l$  and  $\rho$  are directly related to the first derivatives of  $G$ ,

$$\langle \theta_c \rangle = -\frac{\partial G}{N \partial \varepsilon_c}, \quad \langle \theta_l \rangle = -\frac{\partial G}{N \partial \varepsilon_l}, \quad \text{and} \quad V = N/\rho = \frac{\partial G}{\partial P}. \quad (3)$$

Thus, we use

$$G|_{\varepsilon_c, \varepsilon_l, P^*} = G|_{\varepsilon_c, \varepsilon_l, P^*} - N(\varepsilon_c - \varepsilon_{s,0})\theta_c - N(\varepsilon_l - \varepsilon_{n,0})\theta_l + \frac{N}{\phi}(P^* - P_0^*)$$

to extrapolate the Gibbs free energy.

| $(\varepsilon_c, P^*)$ | $\phi_{\text{LDL}}$ | $\phi_{\text{HDL}}$ | $\theta_{s,\text{LDL}}$ | $\theta_{s,\text{HDL}}$ | $\theta_{n,\text{LDL}}$ | $\theta_{n,\text{HDL}}$ | $ \Delta G/k_B T $ |
|------------------------|---------------------|---------------------|-------------------------|-------------------------|-------------------------|-------------------------|--------------------|
| (0.286, 2.61877)       | 0.3158              | 0.3566              | -11.9277                | -48.996                 | -5.4618                 | -13.6145                | 0.06               |
| (0.325, 0.43285)       | 0.1672              | 0.2638              | -7.7509                 | -52.1284                | -3.0612                 | -13.6145                | 0.031              |
| (0.350, 0.08837)       | 0.0788              | 0.1969              | -8.5714                 | -50.5622                | -1.8367                 | -13.0523                | 8.218              |
| (0.370, 0.04538)       | 0.0368              | 0.1486              | -1.2245                 | -45.3413                | -0.6122                 | -11.3655                | 1.194              |
| (0.380, 0.02184)       | 0.0367              | 0.1304              | -15.9183                | -46.3855                | -3.2129                 | -11.6466                | 0.847              |

TABLE I. Interaction strength  $\varepsilon_c$  and reduced pressure  $P^* = PV_{\text{monomer}}$  of liquid–liquid coexistence, and location of the coexisting phases in terms of the density  $\phi$ , crystalline order parameter  $\theta_c$ , and fluid-like order parameter  $\theta_l$ . Rows correspond to separate WTMetaD/Umbrella sampling simulations of  $N = 1024$  proteins. In the last column, we indicate the absolute value  $|\Delta G|$  of the Gibbs free energy difference after reweighting. Deviations from  $\Delta G = 0$  indicate remaining error of the reweighting procedure or inaccurate starting guesses.

## 2. Location of minima and reweighting of the GFES

To find all minima in the GFES, we use a stochastic minimization procedure, basin-hopping, which was originally designed to locate the global minimum on a high-dimensional potential energy surface.<sup>31</sup> Basin-hopping is a two-level scheme in which a random walk on the surface is performed that explores nearby local minima using steepest descent at every step. Here, we use it to re-sample the GFES in the neighborhood of an initial guess for the location of the low- or high-density liquid state. We use a simplex algorithm [`scipy.optimize.minimize(method='nelder-mead')`]<sup>32</sup> to perform the local minimization. We leverage `scipy.optimize.basinhopping()`, which implements the random walk *via* a Metropolis Monte Carlo (MC) scheme. The result of every local minimization and effective sampling temperature  $T$  define the Metropolis acceptance probability. We adjust  $T$  to ensure ergodicity. During the MC updates, we keep track of the minima visited, and subsequently cluster them using using a Gaussian mixture model [`sklearn.BayesianGaussianMixture()`]<sup>33</sup> with  $n = 2$  components corresponding to the two liquid states. The cluster means determine the location and value of the Gibbs free energy minima as initial guesses for a final local minimization step. We iteratively minimize the absolute value  $|\Delta G|$  of their difference, and update the minima at every iteration. We thus *semi-automatically* obtain the reduced pressure  $P_{\text{coex}}^*$  at coexistence from an initial guess that we infer, *e.g.*, from thermodynamic integration (Sec. III B 1).

We checked convergence of the GFES by performing Umbrella sampling on top of the bias potential from well tempered Metadynamics, using 1000 Umbrella sampling windows per state point (10 per dimension). Fig. 3 shows that the qualitative features (LDL, HDL, crystal) revealed by well-tempered metadynamics are unchanged after applying Umbrella sampling correction.<sup>34</sup> We projected the three-dimensional GFES in two dimensions by collapsing two of the collective variables,  $\theta_s$  and  $\theta_n$  onto a linear combination determined by PCA.

## B. Thermodynamic integration of the Helmholtz free energy

We validate the results from WTMetaD simulations using thermodynamic integration of the Helmholtz free energy, which we obtain from the unbiased simulations that produce the order parameter values of Fig. 2.

### 1. Liquid–liquid coexistence from thermodynamic integration of the equation of state

Fig. 4 shows an example of the equation of state in NVT simulations of the patchy shape model, exhibiting liquid–liquid coexistence. We integrate the equation of state along a thermodynamic path that consists of an isochor and an isotherm. The isochor starts from a dilute density  $\phi_0 \equiv \rho_0 V_{\text{monomer}} = 0.02$  and value of  $\varepsilon_{s,0} = 0.25$  above fluid–solid coexistence, and ends at  $(\varepsilon, \phi_0)$ . The isotherm then takes this state point to the final point  $(\varepsilon, \phi)$  in the phase diagram. The change in Helmholtz free energy along that two-segment path (at constant  $\varepsilon_l/\varepsilon_c$ ) is

$$\Delta F_{ex} = \Delta F_1 + \Delta F_2, \quad (4)$$

where

$$\Delta F_1 = -N \int_{\varepsilon_0}^{\varepsilon} d\varepsilon' \left( \langle \theta_c \rangle + \frac{\varepsilon_l}{\varepsilon_c} \langle \theta_l \rangle \right), \quad (5)$$

$$\Delta F_2 = N \int_{\rho_0}^{\rho} d\rho' (\langle P(\rho') \rangle - \rho'). \quad (6)$$

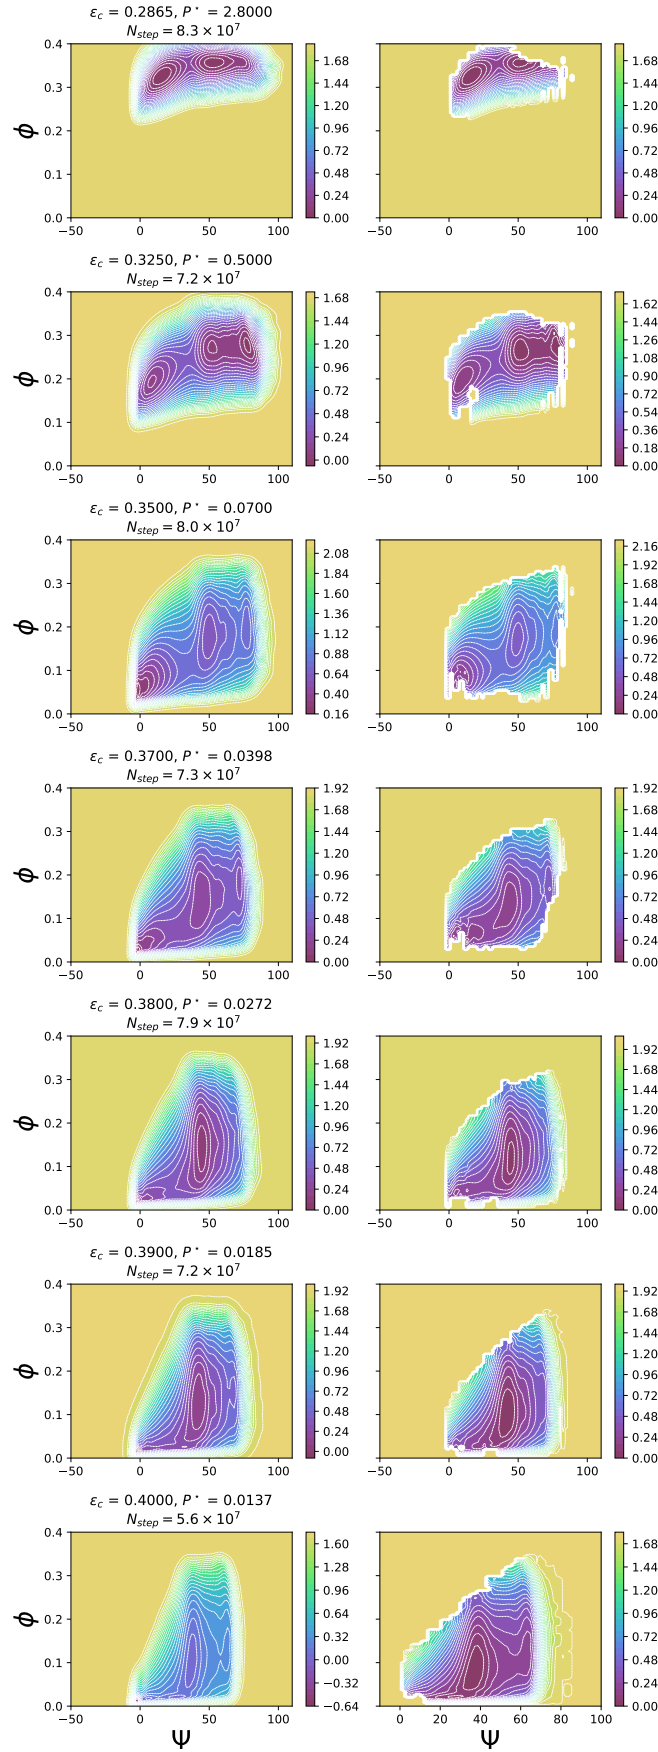

FIG. 3. Gibbs free energy surfaces (GFES)  $g = G/N$  from well-tempered metadynamics (left column) and from Umbrella sampling (right column)

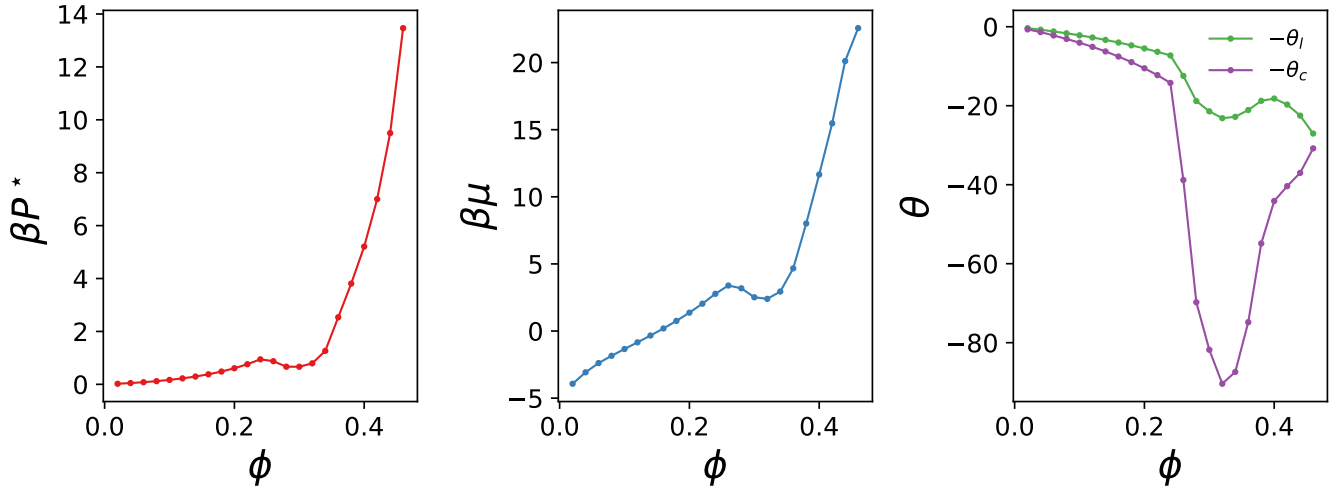

FIG. 4. Equation of state of the patchy shape model at  $\varepsilon_c = 0.3$ ,  $\varepsilon_c/\varepsilon_l = 0.5$ , from NVT simulations with  $N = 8192$  proteins. The densities of the two coexisting metastable liquids for this state point are  $\phi_{\text{LDL}} = 0.256$  and  $\phi_{\text{HDL}} = 0.299$ . *Left*: Reduced pressure  $P^* = PV_{\text{monomer}}$  vs. density  $\phi = \rho V_{\text{monomer}}$ . *Center*: Chemical potential  $\mu = df/d\phi$  from thermodynamic integration of the reduced Helmholtz free energy density  $f = \phi F/N$ . *Right*: Crystal (native) and liquid (non-native) order parameters,  $\theta_c$  and  $\theta_l$ .

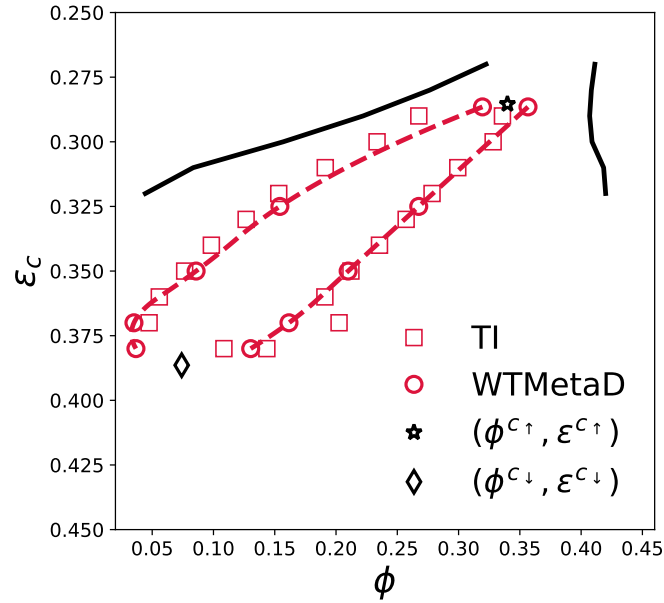

FIG. 5. Comparison between thermodynamic integration (TI, squares) and well-tempered metadynamics (WTMetaD, circles) to locate the liquid–liquid coexistence in the interaction strength–density ( $\varepsilon_c$ – $\phi$ ) plane, for a model with  $\varepsilon_c/\varepsilon_l = 0.5$ . The upper and lower critical points are demarcated by an asterisk, and a diamond respectively. The solid curves are the liquidus and solidus curves, respectively. The dashed curve is an interpolation of the WTMetaD data.

By solving for the two densities that satisfy the equilibrium conditions of equal pressure  $P_{\text{LDL}} = P_{\text{HDL}}$  and chemical potential  $\mu_{\text{LDL}} = \mu_{\text{HDL}}$ , we obtain the binodal limits shown in Fig. 5, which are in satisfactory agreement with those obtained from WTMetaD (Sec. III A).

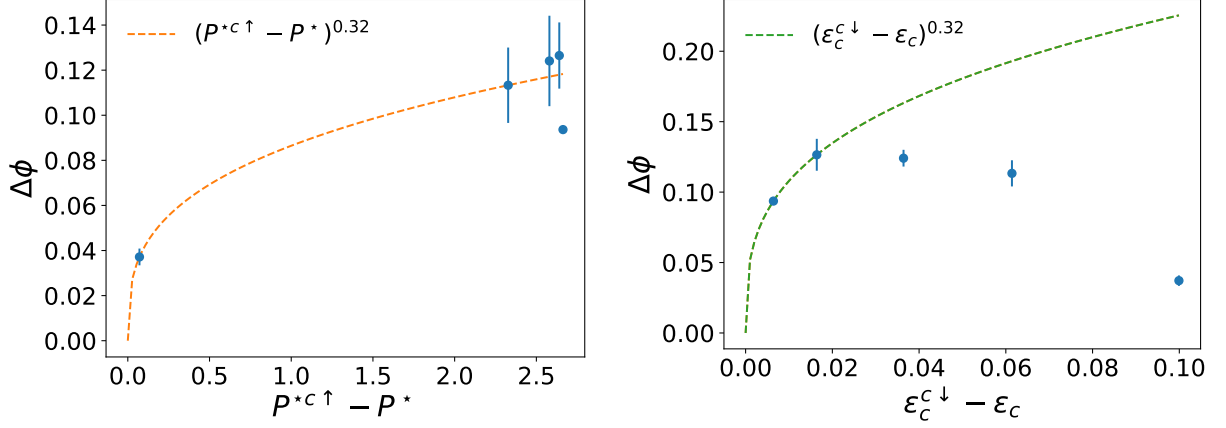

FIG. 6. Estimation of the upper and lower critical points. We plot the density difference  $\Delta\Phi$  between the two liquid phases *vs.* the difference of pressure  $P^*$  to the critical pressure  $P^{*c\uparrow}$  for the upper critical point, and *vs.* the difference to the critical interaction strength  $\varepsilon_c^{c\downarrow}$  for the lower critical point. Curves are fits of the data close to their critical points to a power law.

### C. Critical points

To estimate the upper and lower critical points, we assume they lie in the three-dimensional Ising universality class and that they are second order, confining the line of first order transitions in the interaction strength– pressure  $(\varepsilon_c - P^*)$  plane. As discussed in the main text, the upper critical point corresponds to a transition driven by enthalpic interactions, and the lower critical point to a transition driven by entropy. This classification becomes apparent from the slope of the coexistence curve in the phase diagram (Fig. 7), where the coexistence curve is approximately horizontal or vertical near the upper or lower critical point, respectively. In other words, the first-order transition is driven by small changes in interaction strength  $\varepsilon_c$  near the upper critical point, and by small changes in pressure  $P^*$  near the lower critical point. Consequently, and in the absence of field mixing,<sup>35</sup> we assume that the second order critical points are approached as  $P^{*c\uparrow} - P^*$  and  $\varepsilon_c^{c\downarrow} - \varepsilon_c$ .

To determine the values of  $P^{*c\uparrow}$  and  $\varepsilon_c^{c\downarrow}$ , we fit the density difference  $\Delta\phi = \phi_{\text{HDL}} - \phi_{\text{LDL}}$  between the two coexisting liquids to

$$\Delta\phi \sim (P^{*c\uparrow} - P^*)^\beta, \quad (\text{upper c.p.}) \quad (7)$$

$$\Delta\phi \sim (\varepsilon_c^{c\downarrow} - \varepsilon_c)^\beta, \quad (\text{lower c.p.}) \quad (8)$$

where  $\beta = 0.32$  is the Ising exponent.<sup>36</sup> We then estimate the critical densities  $\phi^{c\uparrow}, \phi^{c\downarrow}$  using the rectilinear diameter law,<sup>7</sup>

$$\frac{1}{2}(\phi_{\text{LDL}} + \phi_{\text{HDL}}) = \phi^{c\uparrow} + A|P^{*c\uparrow} - P^*| \quad (\text{upper c.p.}) \quad (9)$$

$$\frac{1}{2}(\phi_{\text{LDL}} + \phi_{\text{HDL}}) = \phi^{c\downarrow} + A|\varepsilon_c^{c\downarrow} - \varepsilon_c| \quad (\text{lower c.p.}) \quad (10)$$

and obtain  $P^{*c\uparrow} = 2.685$ ,  $\varepsilon_c^{c\uparrow} = 0.285$ , and  $P^{*c\downarrow} = 0.00736$ ,  $\varepsilon_c^{c\downarrow} = 0.386$ . For the densities we get  $\phi^{c\uparrow} = 0.346$  and  $\phi^{c\downarrow} = 0.074$  (Fig. 6).

### D. Fluid–solid coexistence

We calculate the fluid–solid coexistence curves using thermodynamic integration of the Gibbs free energy. We use the Frenkel–Ladd harmonic potential method (Sec. IIID 1) to compute the solid Gibbs free energy. We obtain an initial guess  $(\varepsilon_c^0, P_0^*)$  on the coexistence curve by comparing with the Gibbs free energy from thermodynamic integration of the isothermal-isobaric (NPT) ensemble (Sec. IIID 2). We then trace the coexistence curve using Gibbs–Duhem integration (Sec. IIID 3).

### 1. Solid free energy using the Frenkel–Ladd method

We use a harmonic potential to fix the particles to their equilibrium positions and orientations in the solid and integrate the potential energy along a path from the Einstein solid to the target crystal structure. Along this path, we simultaneously reduce the spring constant to zero and increase the strength of all interactions to their final values, according to Frenkel–Ladd method,<sup>37</sup> as described by Haji-Akbari *et al.*<sup>8</sup> and in Ref.<sup>7</sup> We implement the method using `hpmc.field.frenkel_ladd_energy()` in the Monte Carlo (HPMC) component of HOOMD-blue.<sup>38</sup>

The Helmholtz free energy of the solid is given by

$$F_{\text{solid}} = F_{\text{ein}} + \Delta F + F_{\text{constrain}} - F_{\text{id}}, \quad (11)$$

where

$$\frac{F_{\text{ein}}}{Nk_B T} = -\frac{3}{2} \frac{N-1}{N} \ln \frac{\pi}{\kappa_t} - \frac{3}{2} \ln \frac{\pi}{\kappa_r} - \ln 2 \quad (12)$$

$$\frac{F_{\text{constrain}}}{Nk_B T} = \ln \frac{\rho}{N} - \frac{3}{2N} \ln N - \frac{3}{2N} \ln \frac{\kappa_t}{2\pi} \quad (13)$$

$$\frac{F_{\text{id}}}{Nk_B T} = \frac{1}{2N} \ln N + \ln \rho - 1 + \frac{1}{2N} \ln 2\pi^2, \quad (14)$$

are the free energy contributions per particle of the Einstein crystal and from constraining the center of mass degree of freedom and of the ideal gas. We denote the stiffness of the harmonic springs for the positional and orientational degrees of freedom by  $\kappa_t$  and  $\kappa_r$ , respectively. To account for the angular degrees of freedom of the ideal gas of anisotropic particles, we use  $A_{\mathbb{S}_3} = 2\pi^2$  as the volume of unit quaternion configuration space in  $F_{\text{id}}$ . In Eq. (11),  $\Delta F$  is the integral along the thermodynamic pathway.

$$\Delta F = \int_{\kappa_{\text{max}}}^{\kappa_{\text{min}}} d\kappa \frac{\langle U_{\text{harmonic}} \rangle}{\kappa} + \int_0^1 d\alpha \frac{\partial U}{\partial \alpha}. \quad (15)$$

Here,  $\alpha$  is a dimensionless factor that scales all interactions (attractive and repulsive), and  $\kappa$  is the spring constant. Using the Helmholtz free energy and

$$g_{\text{ex}} \equiv \frac{G_{\text{solid,ex}}}{N} = \mu_{\text{ex}} = F_{\text{solid}} + P/\rho - k_B T, \quad (16)$$

we calculate the excess chemical potential, which is the excess Gibbs free energy  $g$  per particle. We use  $g_{\text{ex}}$  for determining fluid-solid equilibrium (see Sec. IIID 2).

### 2. Equation of state from isothermal-isobaric (NPT) simulations

To obtain the chemical potential  $g$  of the disordered phase, we compute the equation of state in NPT simulations of  $N = 512$  proteins at 2,970 state points. Fig. 7 shows a phase diagram for  $\varepsilon_l/\varepsilon_c = 0.5$ , where the squares are colored by order parameter  $\theta_c$ . High values of the order parameter occur predominantly directly below the *liquid–liquid* coexistence curve and indicate that the HDL phase predicts crystallization (see also discussion of the NVT data in Fig. 2). We integrate the equation of state to obtain the chemical potential  $g$ , first along an isobar and then along an isotherm, in analogy to Sec. IIIB 1 for the Helmholtz free energy. The condition  $g_{\text{solid}} = g_{\text{fluid}}$  determines the initial guess of the coexistence pressure  $P_{\text{coex}}^*$ .

### 3. Fluid–solid equilibrium from Gibbs–Duhem integration

We use Kofke’s Hamiltonian Gibbs–Duhem integration technique<sup>9,39</sup> (as described in Ref.<sup>10</sup>) to trace the the liquidus and solidus curves shown in Fig. 2. We integrate the following generalized Clausius–Clapeyron equation

$$\frac{dP_{\text{coex}}}{d\varepsilon_c} = -\frac{\langle \partial u_{\text{solid}} / \partial \varepsilon_c \rangle_{N, P^*, \varepsilon_c} - \langle \partial u_{\text{fluid}} / \partial \varepsilon_c \rangle_{N, P^*, \varepsilon_c}}{v_{\text{solid}} - v_{\text{fluid}}}, \quad (17)$$

Here,  $v = V/N$  is the volume available to a particle in the each phase, and the energy derivatives per particle are given  $\partial u / \partial \varepsilon_c = -\theta_c$  and  $\partial u / \partial \varepsilon_l = -\theta_l$ . We compute  $dP^*/d\varepsilon_c$  in a coupled simulation of two systems at coexistence,

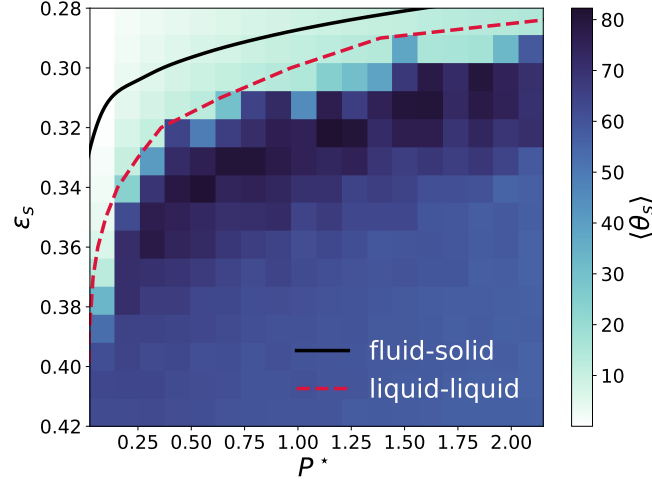

FIG. 7. Phase diagram in the interaction strength–pressure ( $\varepsilon_c - P^*$ ) plane from constant pressure (NPT) simulations of  $N = 512$  proteins, at  $\varepsilon_l/\varepsilon_c = 0.5$ . The squares are colored by the crystalline order parameter  $\langle \theta_c \rangle = -\langle U_c \rangle / N\varepsilon_c$ .

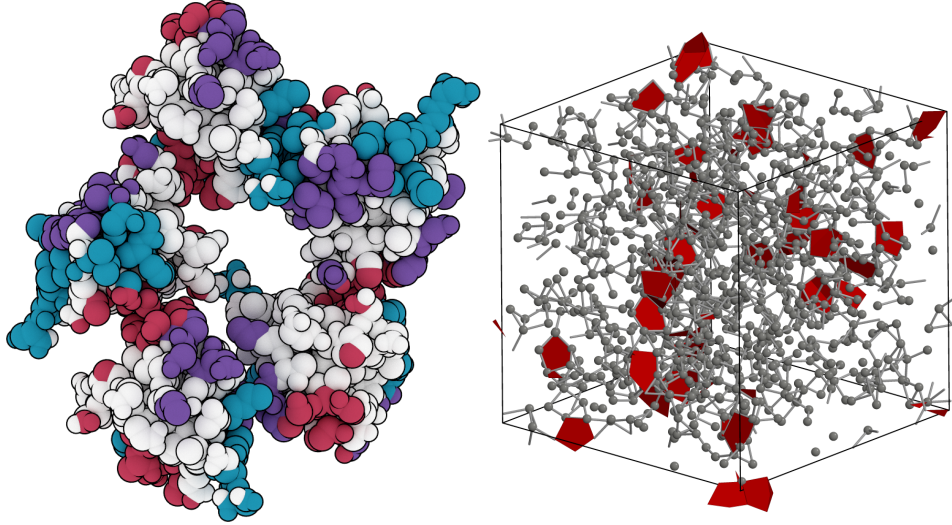

FIG. 8. Observation of ring-shaped prenucleation motifs in the high density liquid phase, stabilized using biased simulations at  $\varepsilon_c = 0.37$ ,  $P^* = 0.0398$ . Bonds up to a nearest neighbor distance cutoff of  $r_{\text{cut}} = 2.5$  nm are included. Left: Typical prenucleation motif. Right: Prenucleation motifs highlighted as pentagons in the bond network of the HDL.

one being disordered and the other one ordered. We initialize the simulation of the solid phase with a self-assembled crystal phase and re-equilibrate it as  $\varepsilon_c$  and  $P^*$  change, and we use the interpolated equation of state of the NPT phase diagram (Sec. III D 2) for the disordered phase, to compute the right hand side of Eq. (17). We use a state point  $(P_0^*, \varepsilon_c^0)$  with equal Gibbs free energies  $G_{\text{solid}} = G_{\text{fluid}}$  for the initial value, which we obtain as described above.

#### IV. PRENUCLEATION MOTIFS IN THE HIGH-DENSITY LIQUID PHASE

In biased simulations, we observe that in the high density liquid typically consists of  $\sim 10\%$  of particles in ring-shaped clusters, which involve all three crystal interfaces. The fraction of ring clusters grows with crystal nucleation, in agreement with the ring cluster being a subunit of the crystal. We do not observe a nucleation-dependent change in the fraction of smaller rings with only four members, as these are not involved in the crystal.

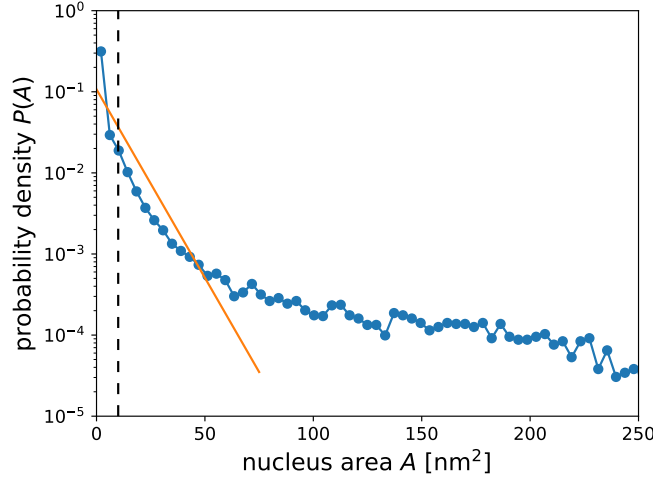

FIG. 9. Distribution  $P(A)$  of the area of pre-critical nuclei for  $\varepsilon_c = 0.3$ ,  $\varepsilon_l/\varepsilon_c = 0.5$  and  $\phi = 0.32$ , together with fit to an exponential distribution (straight line in semi-logarithmic representation).

## V. CHARACTERIZATION OF THE SURFACE TENSION

We determine the fluid–solid surface tension  $\gamma$  from an analysis of pre-critical clusters in 3,680 NVT trajectories. We define clusters by their matching nearest-neighbor bond environments as described in **Methods**, using a distance cut-off of  $r_{\text{cut}} = 5.0$  nm to account for all three protein crystal interfaces. As in Ref.,<sup>12</sup> we assume classical nucleation theory to hold and fit the distribution of cluster areas  $P(A)$  to an exponential decay  $\exp(-\gamma A)$ , as demonstrated in Fig. 9. Clusters with very small area  $A \lesssim 5 \text{ nm}^2$  are slightly overrepresented, but not filtered out; likewise, we opted not to filter out deviations from perfect exponential decay at large cluster areas (and with small probabilities) and accept the  $\gamma$  value from an exponential fit without further manipulation.

- 
- <sup>1</sup> R. Bau, *et al.*, *Journal of Biological Inorganic Chemistry* **3**, 484 (1998).
  - <sup>2</sup> A. Prli, *et al.*, *Bioinformatics* **28**, 2693 (2012).
  - <sup>3</sup> <http://www.biojava.org>.
  - <sup>4</sup> D. Fusco, J. J. Headd, A. De Simone, J. Wang, P. Charbonneau, *Soft matter* **10**, 290 (2014).
  - <sup>5</sup> M. F. Sanner, A. J. Olson, J.-C. Spohner, *Proceedings of the eleventh annual symposium on Computational geometry - SCG '95* (ACM Press, New York, New York, USA, 1995), pp. 406–407.
  - <sup>6</sup> J. D. Weeks, *J. Chem. Phys.* **54**, 5237 (1971).
  - <sup>7</sup> D. Frenkel, B. Smit, *Understanding molecular simulation: From algorithms to applications* (Academic Press, San Diego, 2002), second edn.
  - <sup>8</sup> A. Haji-Akbari, M. Engel, S. C. Glotzer, *The Journal of Chemical Physics* **135**, 194101 (2011).
  - <sup>9</sup> D. A. Kofke, *The Journal of Chemical Physics* **98**, 4149 (1993).
  - <sup>10</sup> C. Vega, E. Sanz, J. L. F. Abascal, E. G. Noya, *Journal of Physics: Condensed Matter* **20**, 153101 (2008).
  - <sup>11</sup> P. M. Piaggi, O. Valsson, M. Parrinello, *Physical Review Letters* **119**, 015701 (2017).
  - <sup>12</sup> U. Gasser, E. R. Weeks, A. Schofield, P. N. Pusey, D. A. Weitz, *Science* **292**, 258 (2001).
  - <sup>13</sup> E. G. Teich, G. van Anders, S. C. Glotzer, *Nature Communications* **10**, 64 (2019).
  - <sup>14</sup> E. S. Harper, M. Spellings, J. Anderson, S. C. Glotzer, harperic/freud: Zenodo DOI release (2016).
  - <sup>15</sup> <http://github.com/glotzerlab/hoomd-blue>.
  - <sup>16</sup> J. A. Anderson, C. D. Lorenz, A. Travesset, *Journal of Computational Physics* **227**, 5342 (2008).
  - <sup>17</sup> J. Glaser, *et al.*, *Computer Physics Communications* **192**, 97 (2015).
  - <sup>18</sup> J. Glaser, S. C. Glotzer, Shape driven phase separation and crystallization of proteins (2019).
  - <sup>19</sup> G. J. Martyna, D. J. Tobias, M. L. Klein, *J. Chem. Phys.* **101**, 4177 (1994).
  - <sup>20</sup> G. J. Martyna, M. E. Tuckerman, D. J. Tobias, M. L. Klein, *Molecular physics* **87**, 1117 (1996).
  - <sup>21</sup> T. F. Miller, *et al.*, *The Journal of Chemical Physics* **116**, 8649 (2002).

- <sup>22</sup> H. Kamberaj, R. J. Low, M. P. Neal, *The Journal of Chemical Physics* **122**, 224114 (2005).
- <sup>23</sup> J. Glaser, P. Schwendeman, J. A. Anderson, S. C. Glotzer, Unified memory in HOOMD-blue improves node-level strong scaling (2019).
- <sup>24</sup> C. S. Adorf, P. M. Dodd, V. Ramasubramani, S. C. Glotzer, *Computational Materials Science* **146**, 220 (2018).
- <sup>25</sup> C. S. Adorf, *et al.*, *Zenodo* (2019).
- <sup>26</sup> A. Laio, M. Parrinello, *Proceedings of the National Academy of Sciences of the United States of America* **99**, 12562 (2002).
- <sup>27</sup> A. Barducci, G. Bussi, M. Parrinello, *Physical Review Letters* **100**, 020603 (2008).
- <sup>28</sup> <http://github.com/jglaser/metadynamics-plugin> .
- <sup>29</sup> J. Glaser, P. Medapuram, T. M. Beardsley, M. W. Matsen, D. C. Morse, *Physical Review Letters* **113**, 068302 (2014).
- <sup>30</sup> <https://github.com/maartenbreddels/ipyvolume.git> .
- <sup>31</sup> D. J. Wales, J. P. K. Doye, *The Journal of Physical Chemistry A* **101**, 5111 (1997).
- <sup>32</sup> <http://www.scipy.org> .
- <sup>33</sup> <http://www.scikit-learn.org> .
- <sup>34</sup> A. L. Ferguson, *Journal of Computational Chemistry* **38**, 1583 (2017).
- <sup>35</sup> P. Virnau, M. Mller, L. G. MacDowell, K. Binder, *The Journal of Chemical Physics* **121**, 2169 (2004).
- <sup>36</sup> J. S. Rowlinson, B. Widom, *Molecular Theory of Capillarity* (Courier Corporation, 2013), reprint edn.
- <sup>37</sup> D. Frenkel, A. J. C. Ladd, *The Journal of Chemical Physics* **81**, 3188 (1984).
- <sup>38</sup> J. A. Anderson, M. Eric Irrgang, S. C. Glotzer, *Computer Physics Communications* **204**, 21 (2016).
- <sup>39</sup> D. A. Kofke, *Molecular physics* **78**, 1331 (1993).
